# Supplementary material for: Value Cards: An Educational Toolkit for Teaching Social Impacts of Machine Learning through Deliberation
Source: arXiv:2010.11411 source file (2023-01-10)
Supplement: Supplementary file 1 [file appendix.tex]

\onecolumn
%\appendix
\setcounter{figure}{0} 

%\section{APPENDIX: The Value Cards Toolkit}

%\subsection{Model Cards}

\begin{figure}[h]
  \centering
    \includegraphics[width=\columnwidth]{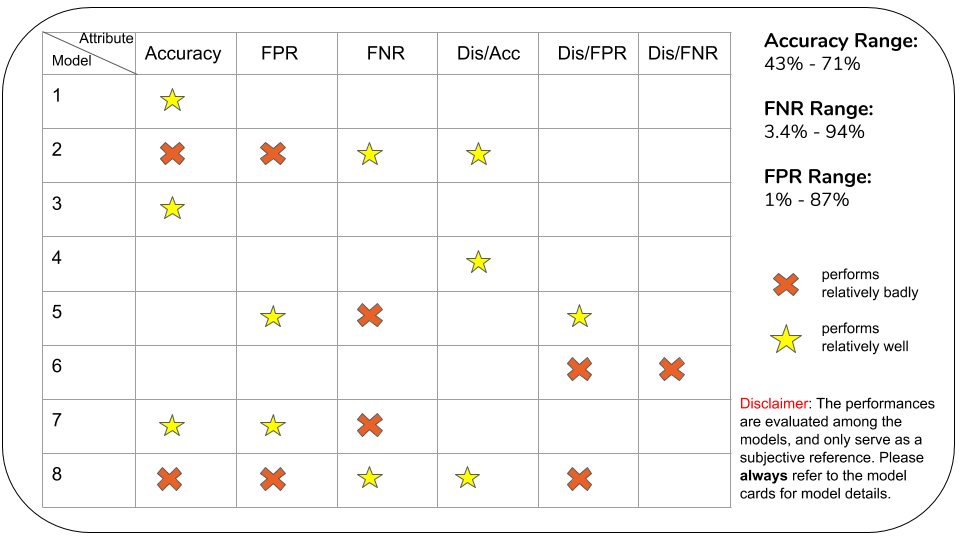}
  \caption{Model Overview}
    
\end{figure}

\begin{figure}[h]
  \centering
    \includegraphics[width=\columnwidth]{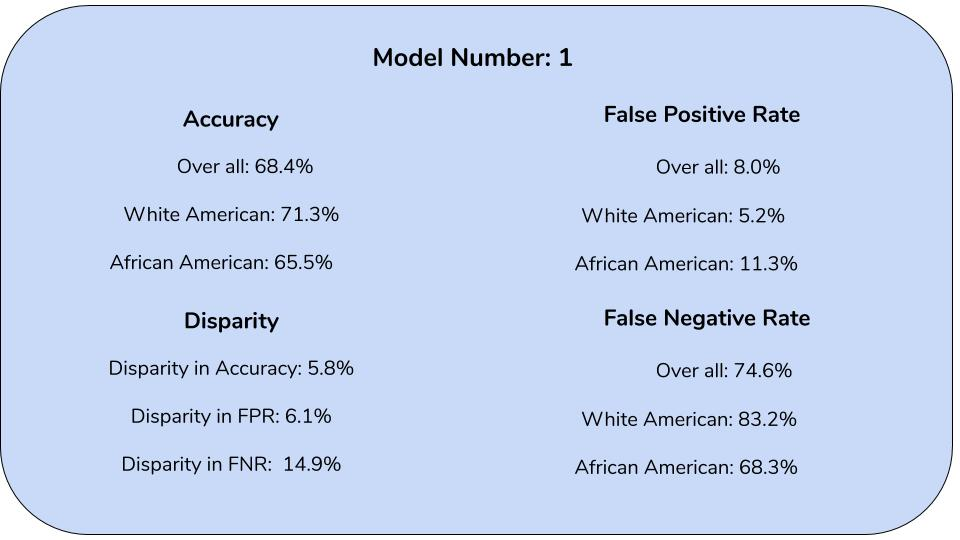}
  \caption{Model 1}
    
\end{figure}

\begin{figure}[h]
  \centering
    \includegraphics[width=\columnwidth]{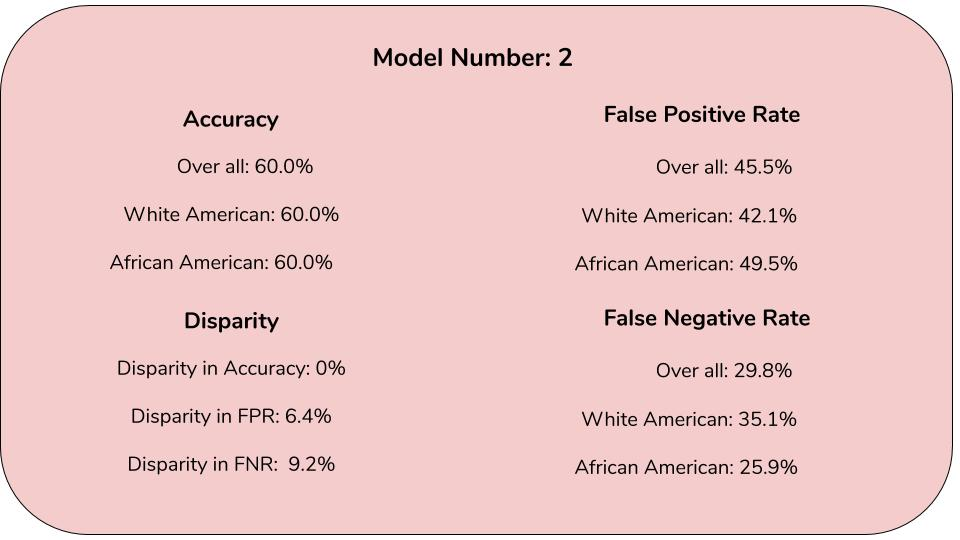}
  \caption{Model 2}
    
\end{figure}

\begin{figure}[h]
  \centering
    \includegraphics[width=\columnwidth]{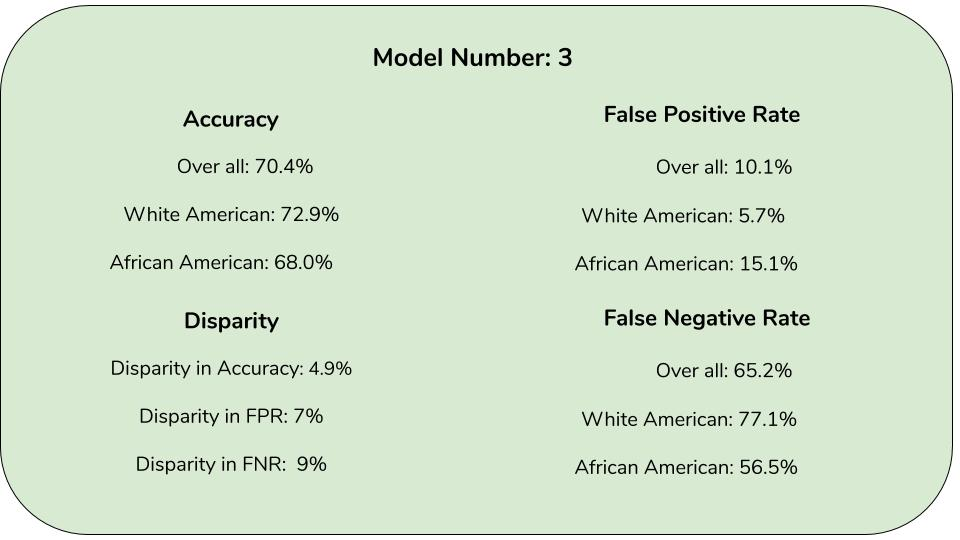}
  \caption{Model 3}
    
\end{figure}

\begin{figure}[h]
  \centering
    \includegraphics[width=\columnwidth]{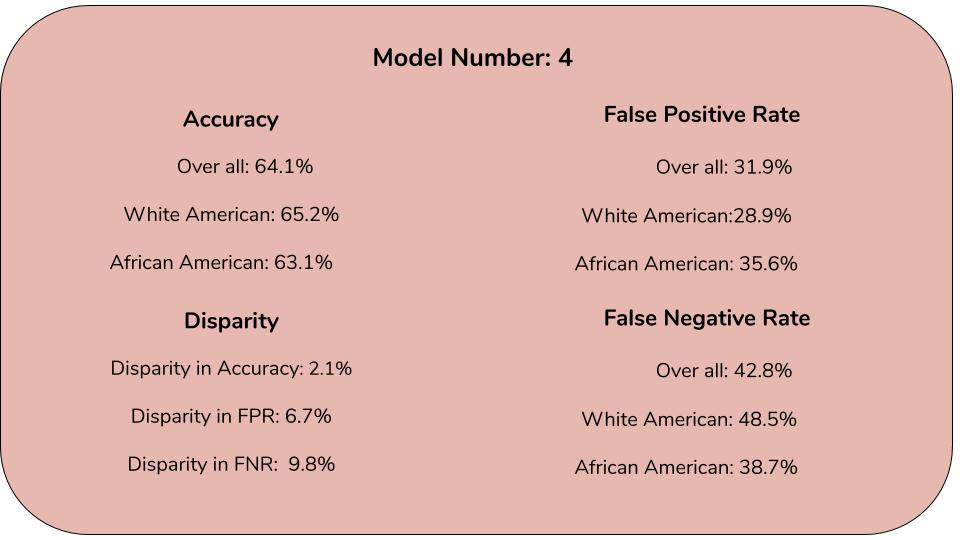}
  \caption{Model 4}
    
\end{figure}

\begin{figure}[h]
  \centering
    \includegraphics[width=\columnwidth]{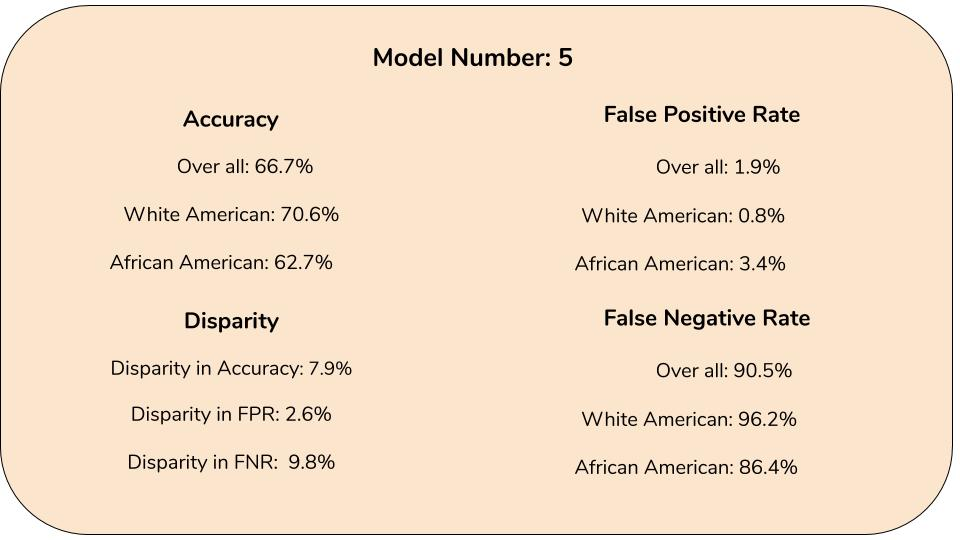}
  \caption{Model 5}
    
\end{figure}

\begin{figure}[h]
  \centering
    \includegraphics[width=\columnwidth]{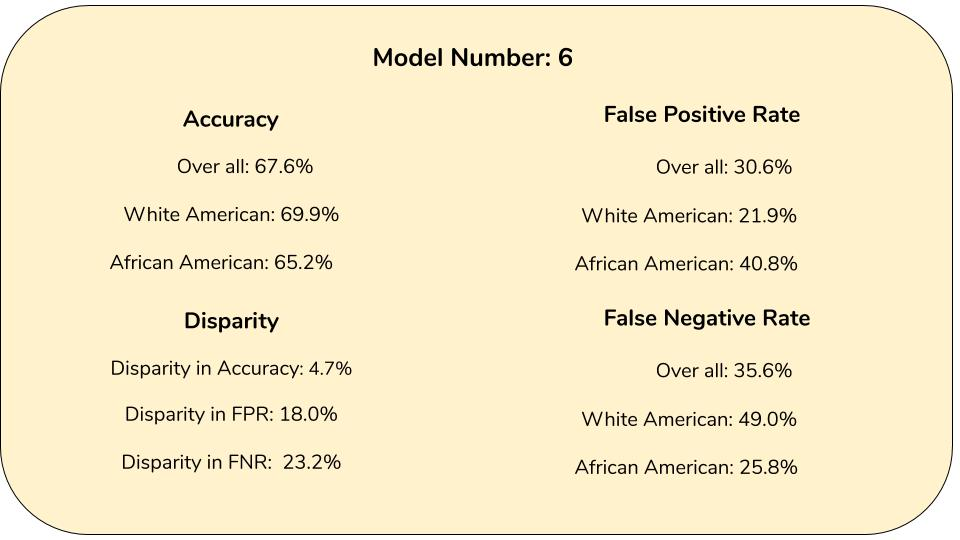}
  \caption{Model 6}
    
\end{figure}

\begin{figure}[h]
  \centering
    \includegraphics[width=\columnwidth]{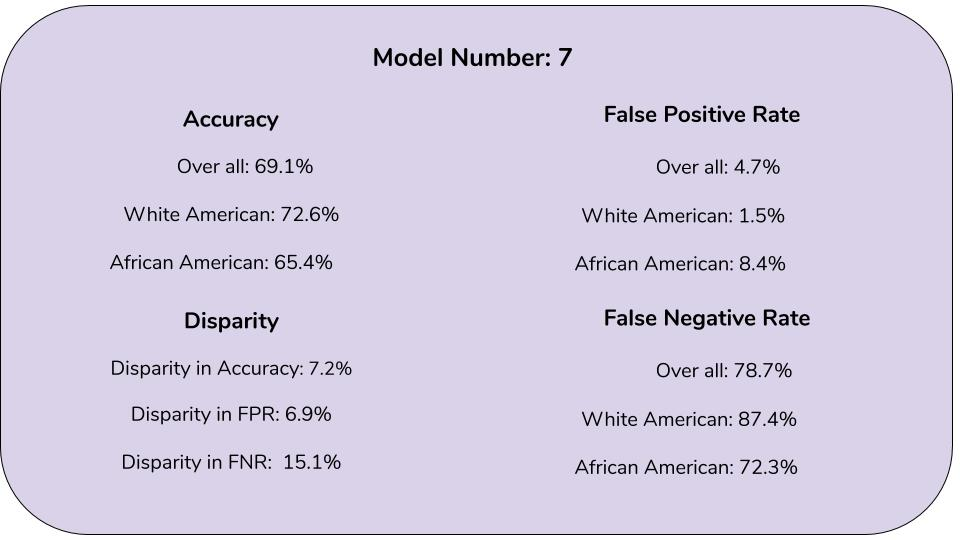}
  \caption{Model 7}
    
\end{figure}

\begin{figure}[h]
  \centering
    \includegraphics[width=\columnwidth]{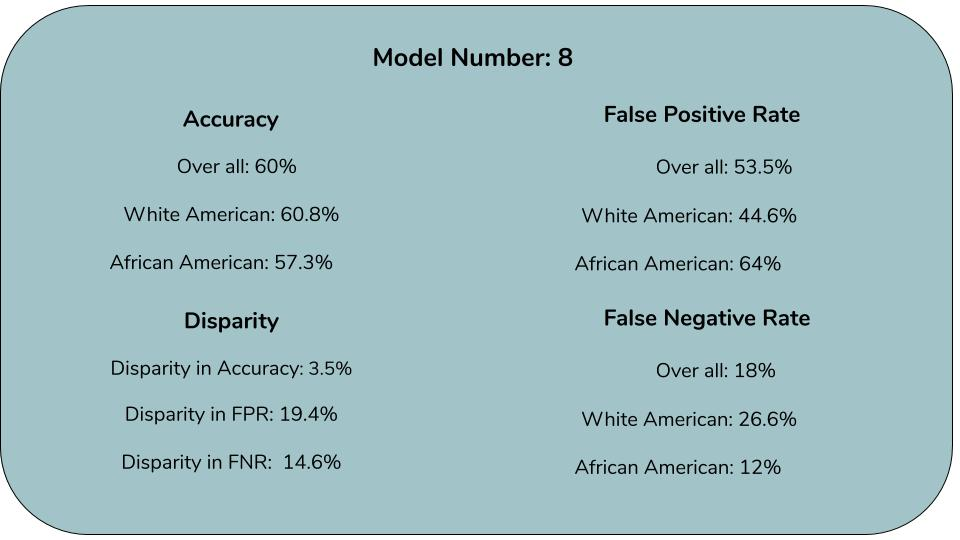}
  \caption{Model 8}
\end{figure}

%\subsection{Persona Cards}

\begin{figure}[h]
  \centering
    \includegraphics[width=\columnwidth]{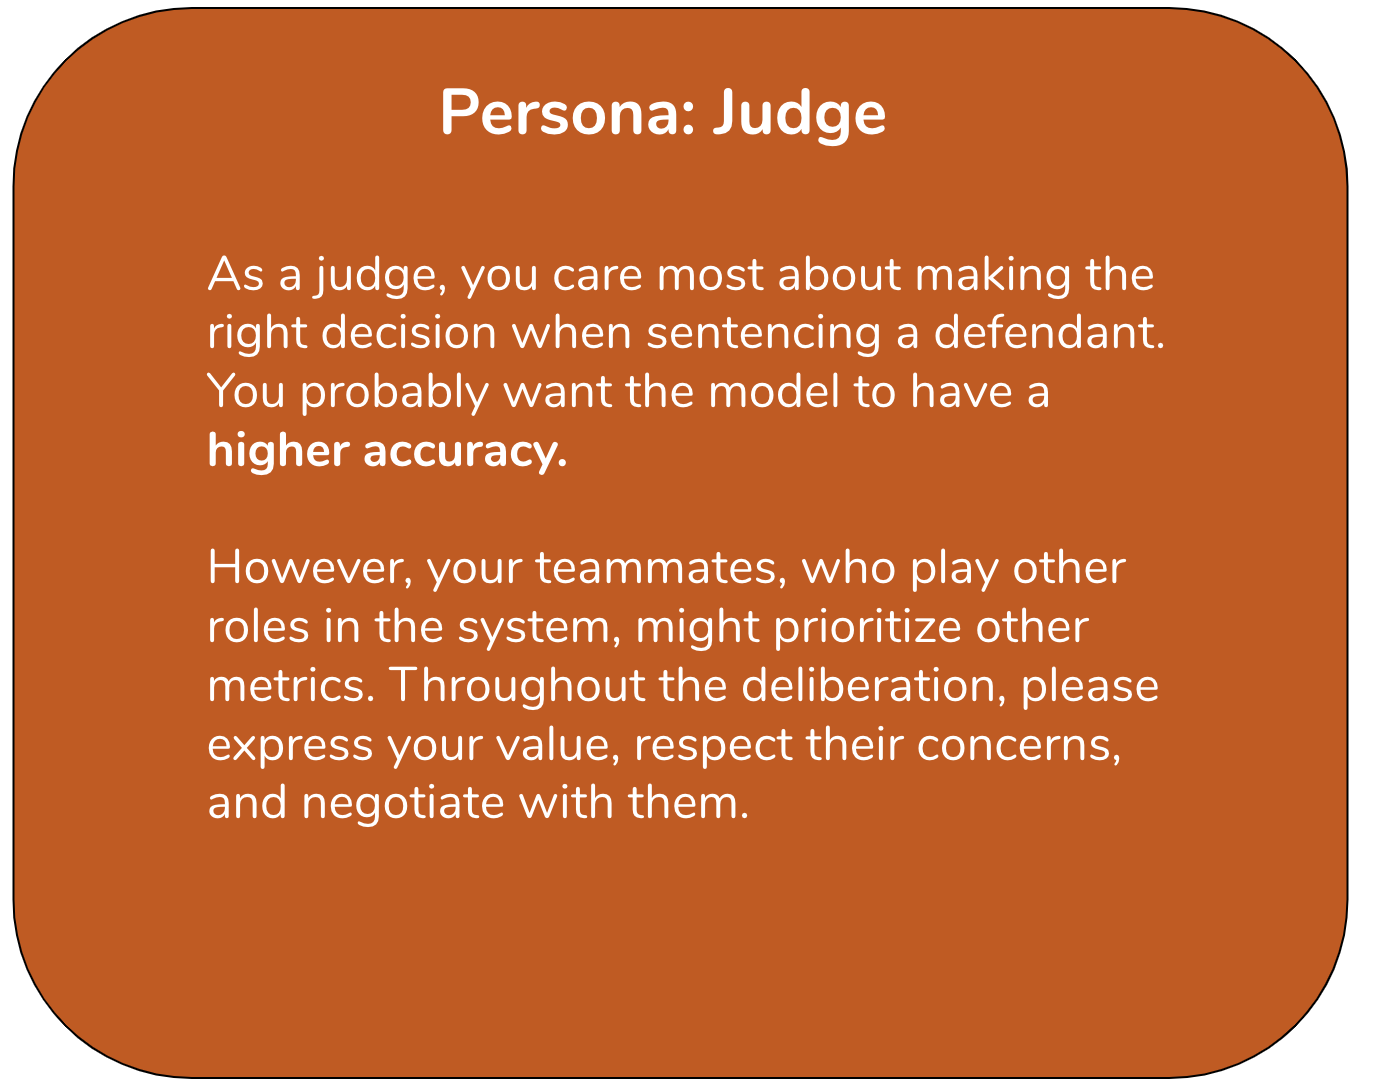}
  \caption{Persona: Judge}
\end{figure}

\begin{figure}[h]
  \centering
    \includegraphics[width=\columnwidth]{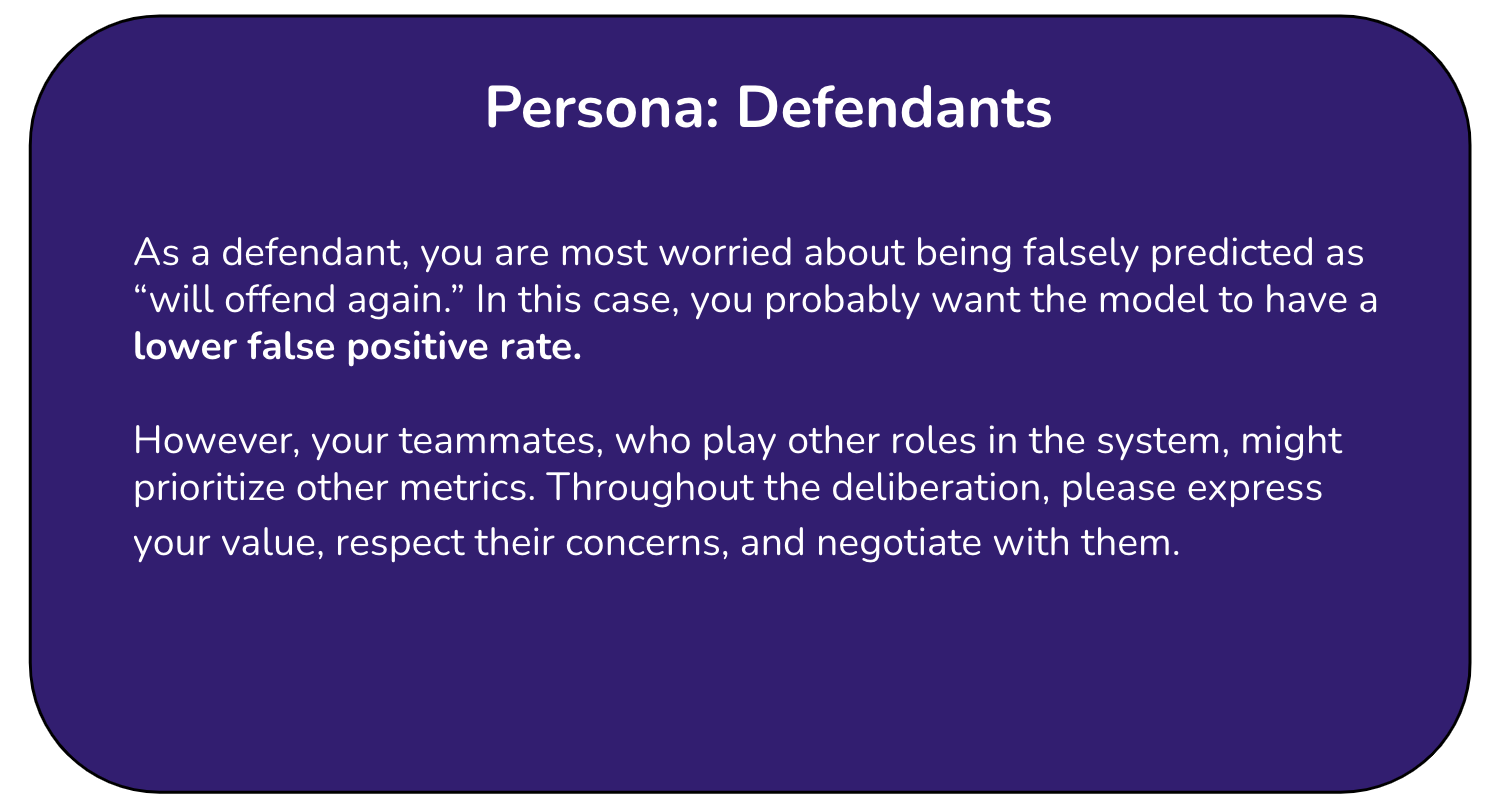}
  \caption{Persona: Defendant}
\end{figure}

\begin{figure}[h]
  \centering
    \includegraphics[width=\columnwidth]{figures/Fairness Advocate.png}
  \caption{Persona: Fairness Advocate}
\end{figure}

\begin{figure}[h]
  \centering
    \includegraphics[width=\columnwidth]{figures/Community members.png}
  \caption{Persona: Community Members}
\end{figure}

%\subsection{Checklist Cards}

\begin{figure}[h]
  \centering
    \includegraphics[width=\columnwidth]{figures/Checklist 1.jpg}
  \caption{Checklist 1}
\end{figure}

\begin{figure}[h]
  \centering
    \includegraphics[width=\columnwidth]{figures/Checklist 2.jpg}
  \caption{Checklist 2}
\end{figure}

\begin{figure}[h]
  \centering
    \includegraphics[width=\columnwidth]{figures/Checklist 3.jpg}
  \caption{Checklist 3}
\end{figure}
